# Supplementary material for: PixHt-Lab: Pixel Height Based Light Effect Generation for Image Compositing
Source: arXiv:2303.00137 source file (2023-02-28)
Supplement: Supplementary file 1 [file 4797.pdf]

# PixHt-Lab: Pixel Height Based Light Effect Generation for Image Compositing Supplementary Materials

Anonymous CVPR submission

Paper ID 4797

## 1. Additional Results

**User study** In addition to the quantitative and qualitative evaluations in the paper, we further applied a user study to quantitatively evaluate the soft shadow quality generated by SSG++ from perception perspective.

The user study is based on the cross-comparison of images generated by GSSN, SSG, and SSN. Besides, we prepared a reference image for participants to identify the shadow and rank the images from the most similar to the least. In total, the user study contains 25 questions. To be fair with SSN, 9 of the 25 questions are experiment1, in which the shadow receiver is always ground plane. Experiment 2 is composed of the other 16 questions, in which the shadow receiver is general shadow receiver. In experiment 2, we just compare SSG and SSG++. We show the image group in random order and positions to 50 participants. The gender statistical distribution of participants is: 81% male, 17% female, 2% not identified. The age distribution of participants is: 71% from the class of $18-30$ years older, 25% from the class of $> 30$ years older, and the rest prefer not to tell.

The average similarity rank score from 1-3 (the lower the score, the more similar the image is) and standard deviation of each model is presented in Fig 1. In experiment 1, SSG++ has an average similarity rank score 1.8; SSG has an average similarity rank score 2.2; SSN has an average similarity rank score 2.0. In experiment 2, SSG++ has an average similarity rank score 1.3; SSG has an average similarity rank score 1.7. In 75% of the questions, the users prefer SSG++, while only in 25% of the questions, the users prefer SSG. Thus, SSG++ performs the best in all the three methods. The T-test for the similarity rank score is significant at 0.001 level, which indicates that images generated from GSSN are significantly more similar to the reference image than images generated from SSG and SSN.

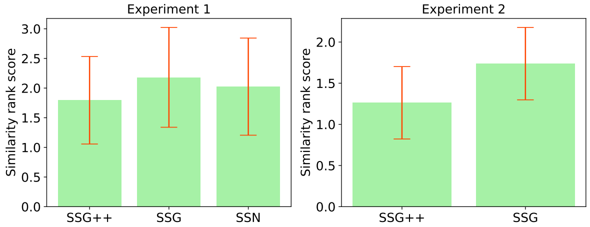


**Figure 1. Ranking score for two experiments (the lower score the better).** The experiments 1 was conducted on the first 9 image groups generated by GSSN, SSG, and SSN. The experiments 2 was conducted on the rest 16 image groups generated by GSSN and SSG.

**More results** The reflection rendering does not assume there is only one cutout object in the scene. We showed more cutout categories in Fig. 2 and in Fig. 3. We further show smooth soft shadow rendering results when the cutouts move and when the softness change in the video supplementary results.

**Comparison with diffusion models** Recent diffusion models [1, 2] show very promising generated images with realistic lighting effects, e.g. reflection, soft shadows, surface shading, etc. Similar to GAN based methods, the common problem for generative methods is that the controllability is limited. PixHt-Lab generate the lighting effects explicitly based on physically based parameters. For example, for the reflection rendering, we use classical physically based parameters, e.g. glossness and Fresnel reflection coefficient. For the soft shadow rendering, we use the size of the area light to control the softness. Another good property for PixHt-Lab is that the change of the results is smooth when the user tweaks the controllable parameters. The smooth transition is demonstrated in the **video** in this supplementary materials.

## References

[1] Robin Rombach, Andreas Blattmann, Dominik Lorenz, Patrick Esser, and Björn Ommer. High-resolution image synthesis with latent diffusion models. In *Proceed-*

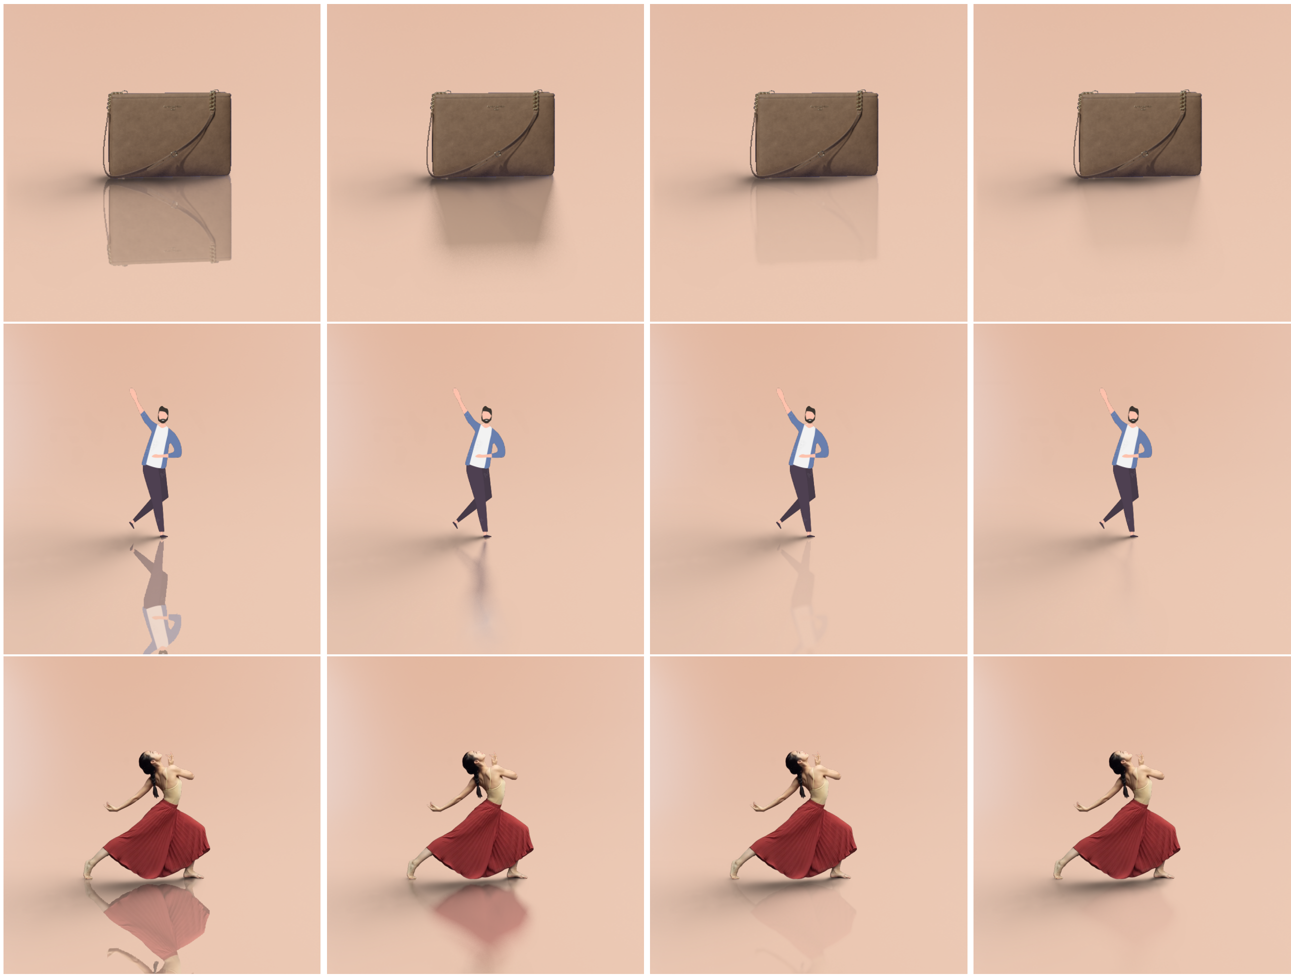

**Figure 2. More reflection.** PixHt-Lab can render reflection for cutouts with product cutout, cartoons, and human dancers.

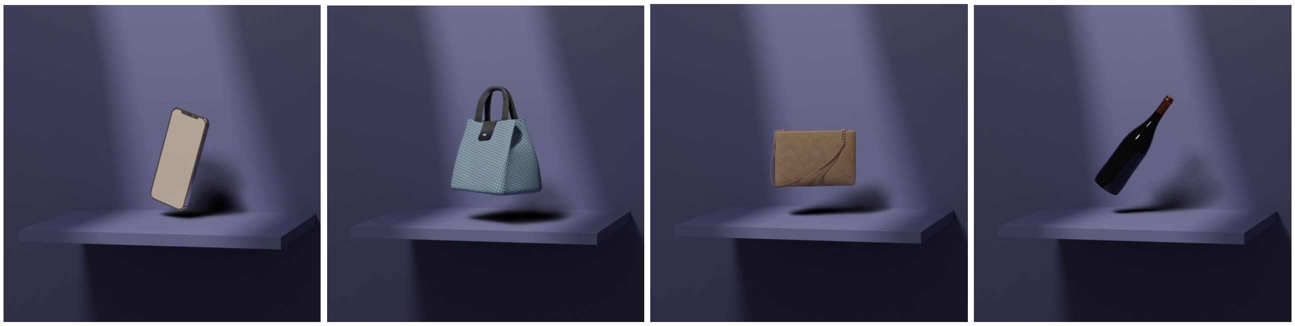

**Figure 3. More shadows.** For different foreground cutouts, PixHt-Lab can render smooth soft shadows on general shadow receivers. Smooth transition example can be found in the video.

*ings of the IEEE/CVF Conference on Computer Vision and Pattern Recognition*, pages 10684–10695, 2022. i

[2] Jascha Sohl-Dickstein, Eric Weiss, Niru Maheswaranathan, and Surya Ganguli. Deep unsupervised learning using nonequilibrium thermodynamics. In *International Conference on Machine Learning*, pages 2256–2265. PMLR, 2015. i
